# Supplementary material for: Prediction targets and surrogate models for active learning of spinel oxygen carriers
Source: arXiv:2611.38088 source file (2026-11-26)
Supplement: Supplementary file 1 [file si_labels.tex]

\makeatletter
\newlabel{SI-si:configs}{{S1}{1}{Strategy and model settings}{si-start}{}}
\newlabel{SI-tab:configs}{{S1}{1}{Strategy identifiers and surrogate training settings. Epoch and iteration values are configured maxima. All runs use a 15\% composition-level validation split}{si-start}{}}
\newlabel{SI-si:screening}{{S2}{3}{Chemical screen}{si-start}{}}
\newlabel{SI-tab:screen_states}{{S2}{3}{Positive oxidation states available to the charge-neutrality screen. The list includes every state with a tabulated Shannon radius, not only states known in spinels}{si-start}{}}
\newlabel{SI-si:oracle}{{S3}{4}{Gibbs energy pipeline}{si-start}{}}
\newlabel{SI-si:quadfit}{{S4}{4}{Quadratic fitting and realization noise}{si-start}{}}
\newlabel{SI-si:stats}{{S5}{4}{Statistical analysis}{si-start}{}}
\newlabel{SI-tab:pipeline}{{S3}{5}{Numerical settings of the Gibbs energy pipeline}{si-start}{}}
\newlabel{SI-tab:quadfit}{{S4}{5}{OTC of the 14 compositions with 20 independent SQS at each vacancy count, converted to the oxygen reference of the active learning runs and ordered by mean quadratic-fit OTC. Mean and sample standard deviation over the 20 curves, in wt.\%}{si-start}{}}
\newlabel{SI-tab:tests}{{S5}{6}{Comparisons between strategies and the test used for each. Each row is a group of comparisons, made separately for mean acquired OTC, run maximum OTC and the mean of the ten best acquisitions unless stated otherwise. Results are in Table~2 of the main text and in Tables~\ref {tab:planned}--\ref {tab:procedures}}{si-start}{}}
\newlabel{SI-tab:runs}{{S6}{7}{Individual run outcomes. OTC values are in wt.\% and exclude the initial dataset. Yield counts new evaluations at or above 6\,wt.\% per nominal budget of 200 selections}{si-start}{}}
\newlabel{SI-tab:planned}{{S7}{8}{Primary contrasts between strategies. Each row compares the strategy in the first column with the one in the second. Differences are the first minus the second in OTC percentage points, with 95\% intervals that are not adjusted for multiplicity. The three clipping contrasts, listed first under each measure, are paired by seed and use paired $t$ tests with four degrees of freedom, and all other contrasts use Welch $t$ tests. $p_{\rm Holm}$ adjusts over the 15 contrasts of each measure. The sensitivity columns give the unadjusted, unpaired Welch probability ($p_{\rm Welch}$), which differs in design from the primary test only for the clipping contrasts, and the Games--Howell probability over all 45 pairs of the ten strategies ($p_{\rm GH}$)}{si-start}{}}
\newlabel{SI-tab:stats-all}{{S8}{9}{All 45 pairwise comparisons for the three run-level measures, as a sensitivity analysis for the primary contrasts of Table~\ref {tab:planned}. Each row compares the strategy in the first column with the one in the second, and differences are the first minus the second in OTC percentage points. $p_{\rm GH}$ is the Games--Howell probability adjusted across the 45 pairs within each measure, not across measures. Simultaneous intervals and Tukey probabilities for selected contrasts are given in Table~\ref {tab:procedures}}{si-start}{}}
\newlabel{SI-tab:procedures}{{S9}{10}{Mean acquired OTC contrasts under each multiplicity procedure. Each row compares the strategy in the first column with the one in the second. Differences are the first minus the second in OTC percentage points, and the interval is the Games--Howell simultaneous 95\% interval. $p_{\rm prim}$ is the Holm-adjusted probability of the primary analysis (Table~\ref {tab:planned}), paired by seed for the clipping contrasts, and a dash marks a contrast outside the primary set. $p_{\rm GH}$ and $p_{\rm Tukey}$ adjust over all 45 pairs of the ten strategies. $p_{\rm WY}$ is a Westfall--Young permutation adjustment over the same 45 pairs. $p_{\rm Holm9}$ restricts the family to these nine selected contrasts and uses exact two-sided rank tests, which cannot reach 0.05 at five runs per strategy (Section~\ref {si:stats}). No contrast is significant under every procedure}{si-start}{}}
\newlabel{SI-si:baselines}{{S6}{11}{Reference baselines and attainable capacity}{si-start}{}}
\newlabel{SI-tab:random-baseline}{{S10}{11}{Random-baseline OTC in wt.\%. The full-sample column summarizes the 500 additional compositions, and the final two columns summarize 20,000 subsets of 200. The maximum-new-OTC row excludes the initial dataset}{si-start}{}}
\newlabel{SI-tab:blocks}{{S11}{11}{Mean attainable ceiling $C(x)$ in wt.\%, and the mean fraction of that ceiling attained, for the new evaluations of each five-cycle block, pooled over the five runs of each strategy. Entries are ceiling / fraction}{si-start}{}}
\newlabel{SI-si:ceiling}{{S7}{11}{Ceiling-only reference}{si-start}{}}
\newlabel{SI-tab:ceiling}{{S12}{12}{Ceiling-only reference runs. OTC and ceiling $C$ in wt.\%, over the 200 new evaluations of each run. $N_{\geq 6}$ counts evaluations at or above 6\wt {}. The last three columns give the percentage of evaluations that release all seven vacancies, release none, and fail the conservative charge scenario~A of Section~\ref {si:screening}}{si-start}{}}
\newlabel{SI-si:holdout}{{S8}{12}{Held-out test of the surrogates}{si-start}{}}
\newlabel{SI-tab:holdout}{{S13}{12}{Held-out test of surrogates trained on the initial dataset, means over five training seeds. Spearman correlations between predicted and evaluated OTC are given for the 500 random-reference compositions, the 1,963 compositions acquired by the MC strategies, all 8,317 compositions acquired by the ten strategies, and the same set without the acquisitions of the model's own strategy family (Excl.\ own). Mean absolute errors (MAE) in wt.\% are for compositions whose evaluated OTC is zero (random set), equals the ceiling, or lies between zero and the ceiling (both on the MC-acquired set). The last column is the mean evaluated OTC of the ten MC-acquired compositions with the highest predictions, against 5.55\wt {} for the ten best evaluated compositions. Clipped denotes the scalar prediction capped at $C$}{si-start}{}}
\newlabel{SI-si:mc_audit}{{S9}{13}{Clipping mass in the MC strategies}{si-start}{}}
\newlabel{SI-si:prediction}{{S10}{13}{Diagnostics}{si-start}{}}
\newlabel{SI-tab:prediction}{{S14}{13}{Error of the logged surrogate prediction relative to the evaluated OTC of the same record, in OTC percentage points, as mean $\pm $ sample standard deviation over five runs. The last column is the percentage of logged predictive means exceeding the selected structure's ceiling (Section~\ref {si:prediction})}{si-start}{}}
\newlabel{SI-si:screens}{{S10}{13}{}{si-start}{}}
\newlabel{SI-tab:charge}{{S15}{14}{Acquisitions retained under the stricter charge scenarios A and B (Section~\ref {si:screening}). Retained fractions are the percentages of new evaluations that pass, averaged over runs, mean OTC is the mean acquired OTC of the passing evaluations in wt.\% averaged over runs, and retained yields count passing evaluations at or above 6\,wt.\% per nominal budget of 200 selections}{si-start}{}}
\newlabel{SI-si:timings}{{S11}{14}{Computational cost}{si-start}{}}
\newlabel{SI-tab:timings}{{S16}{14}{Estimated GPU-seconds per acquisition cycle by workflow stage. Entries are medians over the five per-run cycle medians, with the run range for the first stage in parentheses. The final column gives the first stage as a percentage of the summed stage medians}{si-start}{}}
\newlabel{SI-si:figures}{{S11}{14}{}{si-start}{}}
\newlabel{SI-fig:s01}{{S1}{15}{\textbf {All individual discovery trajectories.} Best OTC found through each cycle, including the initial dataset, for each of the 50 runs. Rows are model families and columns are targets, and the dashed gray line is the initial maximum. MC was not run with Gibbs targets. Panel k shows the five ceiling-only reference runs (Section~\ref {si:ceiling})}{si-start}{}}
\newlabel{SI-fig:s02}{{S2}{16}{\textbf {Run outcomes.} Mean acquired OTC (a), maximum acquired OTC (b) and mean OTC of the ten best acquisitions (c), excluding the initial dataset. Each strategy shows its five runs and a black tick at their mean. Vertical offsets within a row only separate the points and carry no meaning. The last row shows the ceiling-only reference (Section~\ref {si:ceiling}), and each axis is broken so that its low values fit without compressing the other rows}{si-start}{}}
\newlabel{SI-fig:s03}{{S3}{17}{\textbf {Acquisition dynamics and upper tails.} \textbf {a--c,} Mean OTC of new evaluations over the trailing five cycles, from cycle 5 onward. \textbf {d--f,} Fraction of acquisitions at or above each threshold from 4.0 to 6.5\wt {} on a linear scale, including zero fractions. Thin curves are individual runs and thick curves the five-run mean. The initial dataset is excluded}{si-start}{}}
\newlabel{SI-fig:s04}{{S4}{17}{\textbf {Selected acquisition scores relative to the ceiling.} Cumulative distributions of the selected score divided by the ceiling of the saved structure for DE (a), GP (b) and MC (c), pooling the 1,000 selections of each strategy. Scores classified as at the ceiling are drawn at exactly one. Clipped MC clips at a separately rounded mass, so its scores can exceed the ceiling (Section~\ref {si:mc_audit})}{si-start}{}}
\newlabel{SI-fig:s05}{{S5}{18}{\textbf {Composition entropy and OTC.} Cation mixing entropy per AB$_2$O$_4$ formula unit, $S_{\mathrm {mix}}/R$ (labeled $S_{\mathrm {conf}}/R$ on the axes) as defined in the main text, against OTC for new acquisitions pooled over the five runs of each strategy (colored) and for the initial dataset (gray), with separately normalized marginal histograms. Formulas acquired in several runs appear once for each run, and OTC $=0$ corresponds to $\Delta v=0$}{si-start}{}}
\newlabel{SI-fig:s06}{{S6}{19}{\textbf {Accuracy of the reactor relation on the acquired sets.} The relation used by the vacancy-input variants is applied to the evaluated AR curves of each run's acquisitions. \textbf {a,} Root mean squared difference from the evaluated FR energies over the eight vacancy counts. \textbf {b,} Mean absolute OTC difference after quadratic fitting. Each point is one run}{si-start}{}}
\makeatother
